# Supplementary material for: Augmentation adversarial training for self-supervised speaker recognition
Source: arXiv:2007.12085 source file (2020-10-30)
Supplement: Supplementary file 1 [file supplementary.tex]

% \clearpage

% \documentclass{article}
% % Example definitions.
% % --------------------

% % if you need to pass options to natbib, use, e.g.:
% %     \PassOptionsToPackage{numbers, compress}{natbib}
% % before loading neurips_2020

% % ready for submission
% % \usepackage{neurips_2020}

% % to compile a preprint version, e.g., for submission to arXiv, add add the
% % [preprint] option:
% %     \usepackage[preprint]{neurips_2020}

% % to compile a camera-ready version, add the [final] option, e.g.:
% %     \usepackage[final]{neurips_2020}

% % to avoid loading the natbib package, add option nonatbib:
% \usepackage[natbib]{neurips_2020}


% \usepackage{amsmath,graphicx}
% \usepackage{amssymb}
% \usepackage{pifont}
% \usepackage{multirow}
% \usepackage{subcaption}
% \usepackage{makecell}
% \usepackage{listings}
% \usepackage{xcolor}
% \usepackage{stix}
% \usepackage{dirtytalk}
% \usepackage{algorithm}
% \usepackage{algpseudocode}
% \renewcommand{\algorithmicrequire}{\textbf{Input:}}

% \usepackage[utf8]{inputenc} % allow utf-8 input
% \usepackage[T1]{fontenc}    % use 8-bit T1 fonts
% \usepackage{hyperref}       % hyperlinks
% \usepackage{url}            % simple URL typesetting
% \usepackage{booktabs}       % professional-quality tables
% \usepackage{amsfonts}       % blackboard math symbols
% \usepackage{nicefrac}       % compact symbols for 1/2, etc.
% \usepackage{microtype}      % microtypography

% \hypersetup{
%     colorlinks=true,
%     linkcolor=purple,
%     filecolor=magenta,      
%     urlcolor=purple,
% }

% \definecolor{codegreen}{rgb}{0,0.6,0}
% \definecolor{codegray}{rgb}{0.5,0.5,0.5}
% \definecolor{codepurple}{rgb}{0.58,0,0.82}
% \definecolor{backcolour}{rgb}{0.95,0.95,0.92}
 
% \lstdefinestyle{mystyle}{
%     backgroundcolor=\color{backcolour},   
%     commentstyle=\color{codegreen},
%     keywordstyle=\color{magenta},
%     numberstyle=\tiny\color{codegray},
%     stringstyle=\color{codepurple},
%     basicstyle=\ttfamily\footnotesize,
%     breakatwhitespace=false,         
%     breaklines=true,                 
%     captionpos=b,                    
%     keepspaces=true,                 
%     numbers=left,                    
%     numbersep=5pt,                  
%     showspaces=false,                
%     showstringspaces=false,
%     showtabs=false,                  
%     tabsize=2,
%     basicstyle=\fontsize{7}{8}\ttfamily
% }
 
% \lstset{style=mystyle}

% \def\x{{\mathbf x}}
% \def\L{{\cal L}}
% \newcommand{\xmark}{\ding{55}}%
% \newcommand{\cmark}{\ding{51}}%
% \newcommand{\ms}{\mathbf{S}}
% \newcommand{\me}{\mathbf{e}}
% \newcommand{\mx}{\mathbf{x}}

% \newcommand{\RR}{\mathbb{R}}

% \newcommand{\todoc}[2]{{\textcolor{#1}{[#2]}}}
% \newcommand{\todored}[1]{\todoc{red}{\textbf{#1}}}
% \newcommand{\todoblue}[1]{\todoc{blue}{#1}}
% \newcommand{\newpara}[1]{\vspace{6pt}\noindent\textbf{#1}}
% \usepackage{array}
% \newcommand{\PreserveBackslash}[1]{\let\temp=\\#1\let\\=\temp}
% \newcolumntype{C}[1]{>{\PreserveBackslash\centering}p{#1}}
% \newcolumntype{R}[1]{>{\PreserveBackslash\raggedleft}p{#1}}
% \newcolumntype{L}[1]{>{\PreserveBackslash\raggedright}p{#1}}
% \newcommand{\spaceor}{\hspace{1.6pt}|\hspace{1.6pt} }
% \newcommand{\spacepm}{\hspace{1.6pt}$\pm$\hspace{1.6pt}}

% \title{Supplementary Material for "Augmentation adversarial training for self-supervised speaker recognition"}

% % The \author macro works with any number of authors. There are two commands
% % used to separate the names and addresses of multiple authors: \And and \AND.
% %
% % Using \And between authors leaves it to LaTeX to determine where to break the
% % lines. Using \AND forces a line break at that point. So, if LaTeX puts 3 of 4
% % authors names on the first line, and the last on the second line, try using
% % \AND instead of \And before the third author name.

% \author{
% \name{Jaesung Huh$^{1}$, Hee Soo Heo$^{1}$, Jingu Kang$^{1}$, Shinji Watanabe$^{2}$, Joon Son Chung$^{1}$} \\
% \address{$^{1}$Naver Corporation, South Korea \\
% $^{2}$Johns Hopkins University, Baltimore, USA \\
% }
% }


% \begin{document}

% \maketitle

% \input{appendix}

% \bibliographystyle{plain}
% \bibliography{shortstrings,mybib,vgg_local,vgg_other}
% \end{document}
